# Supplementary material for: Superconductivity behavior in epitaxial TiN films points at surface magnetic disorder
Source: arXiv:1903.05009 source file (2019-11-05)
Supplement: Supplementary file 1 [file Supplemental_material_TiN.pdf]

# Supplemental Material for Superconductivity behavior in epitaxial TiN films points to surface magnetic disorder

N.A. Saveskul,[1] N.A. Titova,[1] E.M. Baeva,[2,1] A.V. Semenov,[1] A.V. Lubenchenko,[3]
S. Saha,[4,5] H. Reddy,[4,5] S. Bogdanov,[4,5] E.E. Marinero,[4,6] V.M. Shalaev,[4,5]
A. Boltasseva,[4,5] V.S. Khrapai,[2,1,7] A.I. Kardakova,[2,1] and G.N. Goltsman[2,1]

[1] *Moscow State University of Education, 29 Malaya Pirogovskaya St, Moscow, 119435, Russia*
[2] *National Research University Higher School of Economics, 20 Myasnitskaya St, Moscow, 101000, Russia*
[3] *National Research University MPEI, Krasnokazarmennaya St., 14, Moscow, 111250, Russia*
[4] *School of Electrical & Computer Engineering and Birck Nanotechnology Center, Purdue University, 1205 West State Street, West Lafayette, Indiana 47907-2057, USA*
[5] *Purdue Quantum Science and Engineering Institute, Purdue University, West Lafayette, Indiana 47907, USA*
[6] *School of Materials Engineeing, Purdue University, 1205 West State Street, West Lafayette, Indiana 47907-2057, USA*
[7] *Insitute of Solid State Physics, 2 Ak. Osipyana St., Chernogolovka, 142432, Russia*

## I. TRANSPORT MEASUREMENTS OF TIN SAMPLES FROM SET 2

Figure 1S displays the temperature dependences of resistance for TiN samples from set 2. The data are presented for thick (200 nm and 100 nm) and ultrathin (4 nm and 3 nm) TiN films. The insets in Fig. 1S show the temperature dependencies of the second critical magnetic field $B_{c2}$, obtained from the shift of the superconducting transition temperature in a perpendicular magnetic field.

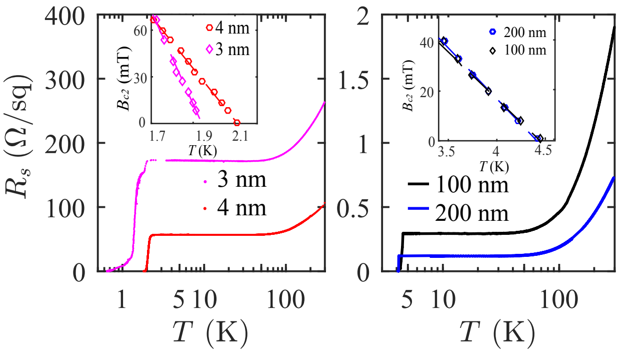


FIG. 1S. **Transport measurements of TiN samples from set 2.** (Left) The temperature dependence of resistance for thick TiN films: 200 nm ($T_c = 4.5$ K) and 100 nm ($T_c = 4.5$ K). (Right) The temperature dependence of resistance for thin TiN films: 4 nm ($T_c = 1.9$ K) and 3 nm ($T_c = 1.4$ K). In the insets, the temperature dependencies of the second critical magnetic field $B_{c2}$, obtained from the shift of the superconducting transition temperature in a perpendicular magnetic field.

## II. XPS ANALYSIS OF TIN FILMS ON $AL_2O_3$ SUBSTRATES

X-ray photoelectron spectroscopy (XPS) is one of the non-destructive methods of thin and ultra-thin films analysis. XPS spectra are obtained by irradiating a material with a beam of X-rays while simultaneously measuring the kinetic energy and number of electrons that escape from the top of the studied material. The chemical and phase depth profiling can be obtained on the base of the method described in Ref. [1].

The XPS studies of the TiN sample were performed using the electron-ion spectroscopy module based on Nanofab 25 (NT-MDT) platform. The setup includes the analysis chamber with an ultrahigh oil-free vacuum ($10^{-7}$ mbar), the X-ray source SPECS XR 50 with Mg anode without a monochromator with an excitation energy 1253.6 eV. The spectra were recorded with an electrostatic hemispherical energy analyzer SPECS Phoibos 225 with a pass energy of 80 eV.

TABLE I. Chemical and phase depth profile of ultra-thin TiN films.

| | Formula | d (nm) | | |
|---|---|---|---|---|
| | | 3 nm | 5 nm | 20 nm |
| 7 | hydrocarbons | 0.7 | 0.6 | 0.6 |
| 6 | $TiO_2$ | 0.4 | 0.4 | 0.5 |
| 5 | $TiO_x$ | 0.5 | 0.5 | 0.5 |
| 4 | $Ti(NO)_x$ | 0.4 | 0.8 | 1.2 |
| 3 | $TiN_x$ | 0.8 | 1.4 | 1.5 |
| 2 | TiN | 1.1 | 2.5 | Not |
| 1 | $AlO_x$ | 1.8 | 2.2 | record |
| 0 | $Al_2O_3$ | Substrate | | |

Figure 2S displays experimental XPS data presented for 5-nm TiN film. The analogous spectrum are also obtained for 3 nm and 20 nm films. Figure 2S shows decomposition of XPS lines of an element of interest (Ti, N, O, Al) into component peaks that reveals presence of different phases in the sample ($TiO_2$, $TiO_x$, $Ti(NO)_x$, $TiN_x$,TiN). The procedure of XPS peaks deconvolution is described in Ref. [1]. The results of the XPS line decomposition allow to extract thicknesses of layers of different phases in the studied TiN sample. The data are presented in Table I.

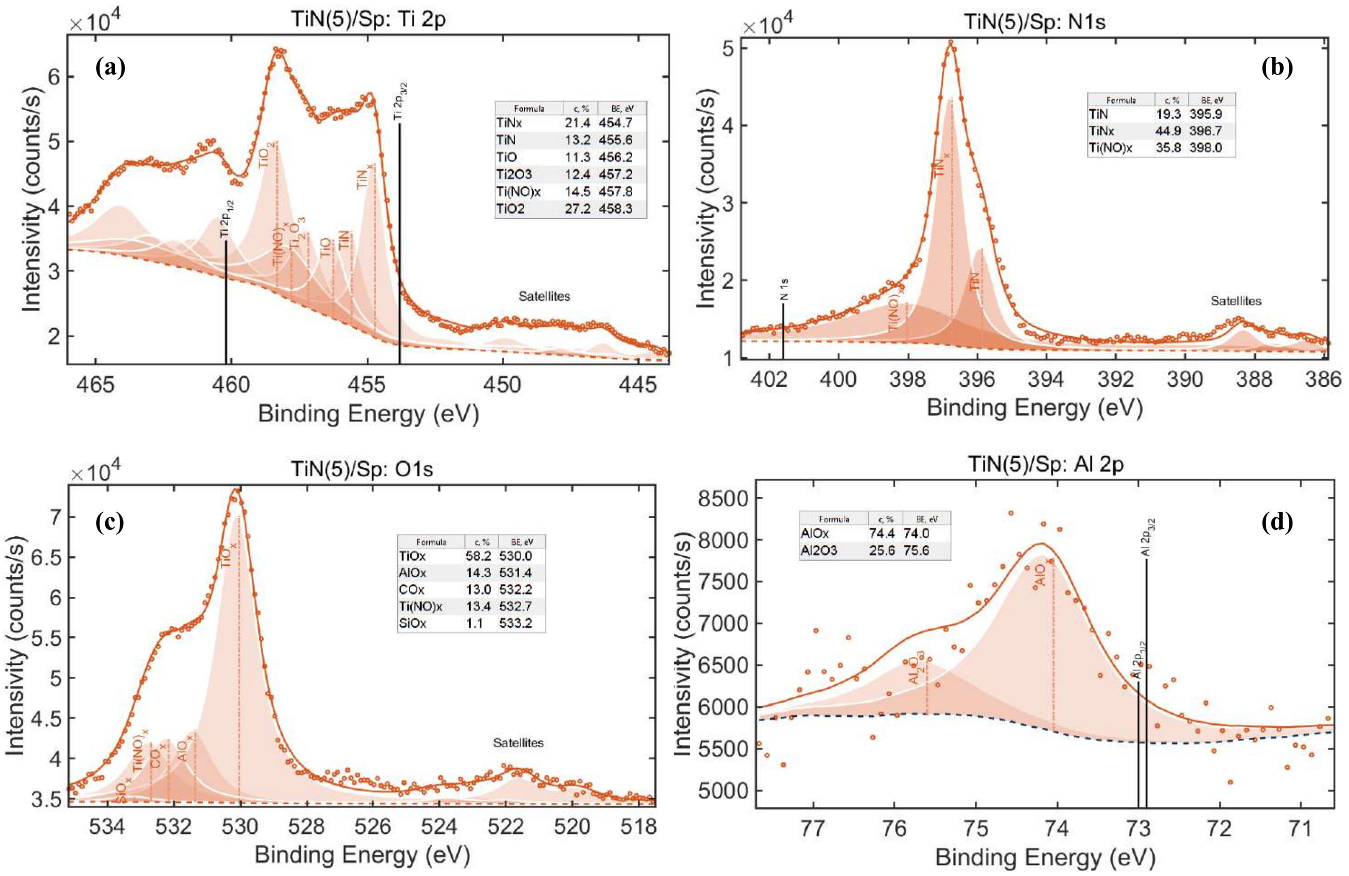


FIG. 2S. **XPS survey spectrum of 5-nm TiN film.** XPS spectra are obtained by irradiating a material with a beam of X-rays while simultaneously measuring the kinetic energy and number of electrons that escape from the top of the material. The XPS data show decomposition of lines into partial peaks: (a) Line Ti 2p, (b) Line N 1s, (c) Line O 1s, (d) Line Al 2p. The peak height is mainly determined by atomic relative concentrations of an element in the sample and proximity of the element to the surface. The figure shows decomposition of XPS lines of elements (Ti, N, O, Al) into component peaks that reveals presence of different phases in the sample ($TiO_2$, $TiO_x$, $Ti(NO)_x$, $TiN_x$, TiN). The results of the XPS line decomposition allow to extract thicknesses of layers of different phases in the studied TiN sample.

## III. GRAIN EFFECTS ON RESIDUAL RESISTIVITY

In thin films, increase the resistivity of the system occur with additional scattering mechanisms. The two fundamental mechanisms are: (i) scattering of electrons at external surfaces or interfaces (the Fuchs-Sondheimer model [2, 3]); (ii) scattering of electrons at grain boundaries (Mayadas-Shatzkes model [4]).

The latter one focuses on the scattering of electrons at grain boundaries, which can be found in polycrystalline materials between several crystallites. The boundaries can be regarded as potential barriers for the travelling electrons, where they can either be reflected or transmitted. The reflection probability of an electron is described by the grain boundary reflection coefficient $R$. The higher $R$, the more electrons are reflected and the higher is the resulting resistivity. Another important factor is the density of the grain boundaries, which is accommodated in the model by the average grain size $D_g$. The conductivity, due to MS-model, can be determined by:

$$\sigma_g = \sigma_0 \cdot f(\alpha), \tag{1}$$

with

$$f(\alpha) = 1 - \frac{3}{2}\alpha + 3\alpha^2 - 3\alpha^3 ln(1+\alpha^{-1}), \tag{2}$$

where $\alpha = (l_0/D_g)\ R/(1-R)$, $\sigma_0$ and $l_0$ are the conductivity and the mean free path inside a grain, respectively.

Mayadas and Shatzkes expanded their model of grain boundary scattering to the case of thin films, and for this purpose the framework of the Fuchs theory was used. The total film conductivity $\sigma_f$ can be calculated by:

$$\sigma_f = \frac{1}{\rho_g} - \frac{6}{\pi\kappa_0\rho_0}\int_0^{\pi/2} d\phi \int_1^{\infty} dt \frac{cos^2\phi}{H^2(t,\phi)}\left(\frac{1}{t^3}-\frac{1}{t^5}\right)\times$$
$$\times \frac{1-e^{-\kappa_0 t H(t,\phi)}}{1-pe^{\kappa_0 t H(t,\phi)}}, \tag{3}$$

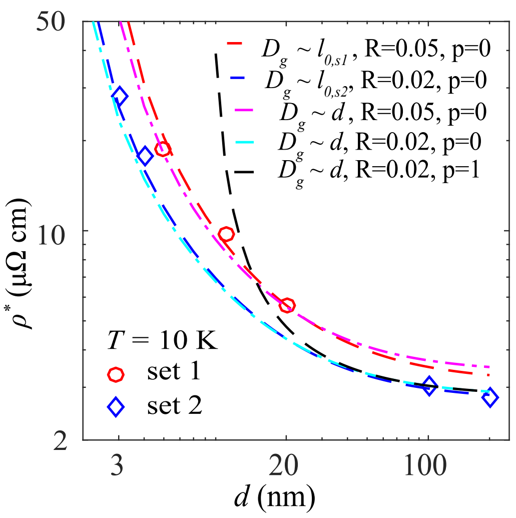


FIG. 3S. **Effect of the scattering at grain boundaries on residual resistivity.** Resistivity ($\rho^*$) as a function of film thickness ($d$). The red circles correspond to data for the set 1, the blue diamonds - for the set 2. The values of resistivity are corrected assuming the dead layer, $\rho_0^* = R_{sq}^{10K}(d - d_{DL})$. The dashed red and blue lines are fits of the MS-model (Eq. 3) assuming columnar grains with $D_g \sim\ l_0$, the reflection coefficient $R < 0.05$ and the limit of diffusive scattering ($p = 0$). The dot-dashed cyan and magenta fits are obtained assuming the spherical grains $D_g \sim\ d$ and the reflection coefficient $R < 0.05$. The dashed black line illustrates the case of specular surface scattering ($p = 1$).

where $\rho_g = \sigma_g^{-1}$, $\rho_0 = \sigma_0^{-1}$, $\kappa_0 = d/l_0$, and $H(t,\phi)$ is defined by

$$H(t,\phi) = 1 + \frac{\alpha}{cos\phi\sqrt{(1-1/t^2)}}.$$

Fig. 3S shows the results of fitting of $\rho(d)$ data using the MS-model that reveals negligible contribution of electron scattering at grain boundaries in the studied TiN films.

## IV. THE TEMPERATURE DEPENDENCE OF FILM RESISTIVITY

The temperature dependent part of $\rho(T)$ can be characterized with the Bloch-Grüneisen formula [5]:

$$\rho_T^{BG}(T) = A\left(\frac{T}{\theta_D}\right)^5 \int_0^{\theta_D/T} \frac{x^5 dx}{(e^x-1)(1-e^{-x})}, \qquad (4)$$

where $A$ is a coupling constant.

Fig. 4S shows temperature dependences of the normalized resistivity, $(\rho - \rho_0)/\rho^{300K}$. The linear term of $\rho(T)$, that corresponds to a high-temperature asymptote, holds down to $T \approx 200$ K (that corresponds to $T \sim \theta_D/3$) for all studied TiN films.

Additionally, we estimated the ratio of the Debye temperature to the Bloch-Grunheisen temperature,

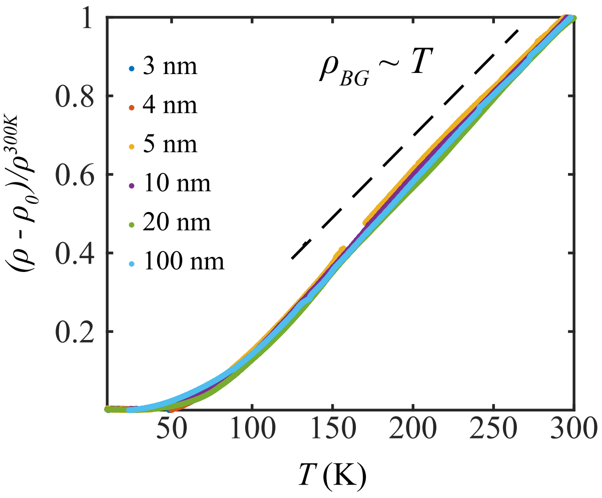


FIG. 4S. **The temperature dependence of film resistivity.** The temperature dependence of the normalized resistivity, $(\rho - \rho_0)/\rho^{300K}$. The data, presented for films of different thicknesses, are fitted with the Bloch-Grüneisen formula (Eq. 4). The fitting parameters are the Debye temperature $\theta_D$ and the material constant $A$. The values of the fitting parameters for TiN films are in the range of $480 - 550$ K for the Debye temperature and $80 - 120\,\mu\Omega cm$ for the material constant $A$.

$\theta_D/T_{BG}$, that can be simplified as $(6\pi^2 N_{ion})^{1/3}/(2k_F) = (N_{ion}/4n)^{1/3}$, where $N_{ion}$ is the atomic number density, $k_F = (3\pi^2 n)^{1/3}$ is the Fermi wave vector, $n$ is the carrier density. Taking $N_{ion} = 1/a^3$ ($a = 0.42$ nm the lattice constant) $= 1.31 \times 10^{22}\,\mathrm{cm}^{-3}$ and $n = 5.25 \times 10^{22}\,\mathrm{cm}^{-3}$, we obtain the ratio $\theta_D/T_{BG} = 0.4$ that corresponds to the case of normal metal scenario [6].

## V. ESTIMATION OF THE FERMI VELOCITY

To characterize the behavior of the conduction electrons, we estimate an average Fermi velocity from experimental values of electron diffusivity and transport scattering time as $v_F = \sqrt{ND/\tau_{tr}}$ (see Figure 5S). Here, $N$ is the dimensionality of the system in terms of diffusive transport. The films with thicknesses $d \leq 20$ nm are considered in 2D regime as the condition $l \geq d$ is satisfied. The electron diffusivity constant can be determined from the slope of the temperature dependencies of the second critical magnetic field $B_{c2}(T)$ at $T = T_c$ using the relation

$$D = -\frac{12k_B}{N\pi e}\left(\frac{dB_{c2}(T)}{dT}\right)^{-1}_{T=T_c}. \qquad (5)$$

The values of electron diffusivity, which we are estimated with Eq.(5), are $15 \pm 2\,\mathrm{cm}^2/\mathrm{s}$, $12 \pm 2\,\mathrm{cm}^2/\mathrm{s}$, $8 \pm 2\,\mathrm{cm}^2/\mathrm{s}$ for 20 nm, 10 nm, and 5 nm, respectively (set 1). For films from set 2 the values of $D$ are $26 \pm 2\,\mathrm{cm}^2/\mathrm{s}$,

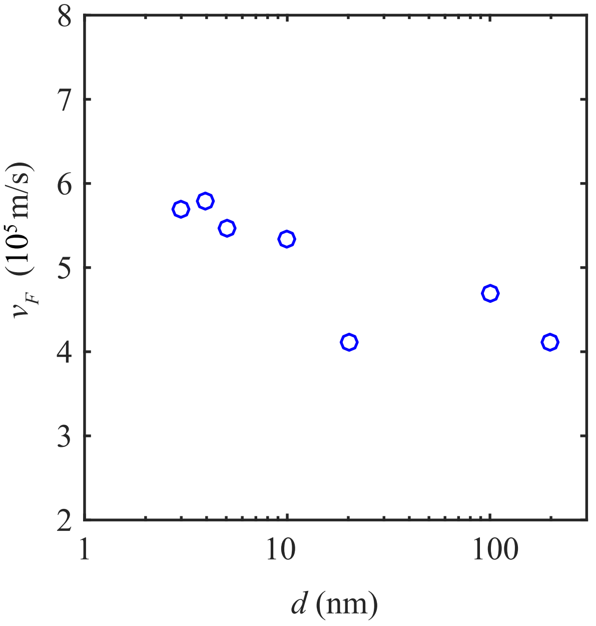


FIG. 5S. **Estimation of the Fermi velocity.** The thickness dependence of the Fermi velocity, $v_F = \sqrt{D\tau_{tr}}$, determined for two sets.

$28 \pm 2\,\mathrm{cm}^2/\mathrm{s}$, $10 \pm 0.5\,\mathrm{cm}^2/\mathrm{s}$, $6 \pm 0.5\,\mathrm{cm}^2/\mathrm{s}$ for 200 nm, 100 nm, 4 nm, and 3 nm, respectively. The transport relaxation time was estimated as $\tau_{tr} = 1/(\rho^{10K}\omega_p^2\varepsilon_0)$ using the experimental values of plasma frequency $\omega_p$ and low temperature resistivity $\rho^{10K}$.


[1] A. V. Lubenchenko, A. A. Batrakov, A. B. Pavolotsky, O. I. Lubenchenko, and D. A. Ivanov, "XPS study of multilayer multicomponent films," Applied Surface Science **427**, 711 – 721 (2018).

[2] K. Fuchs, "The conductivity of thin metallic films according to the electron theory of metals," Mathematical Proceedings of the Cambridge Philosophical Society **34**, 100–108 (1938).

[3] E.H. Sondheimer, "The mean free path of electrons in metals," Advances in Physics **1**, 1–42 (1952).

[4] A. F. Mayadas, M. Shatzkes, and J. F. Janak, "Electrical resistivity model for polycrystalline films: The case of specular reflection at external surfaces," Applied Physics Letters **14**, 345–347 (1969).

[5] J. M. Ziman, *Electrons and Phonons: The Theory of Transport Phenomena in Solids* (Oxford University Press, New York, 2001).

[6] E. H. Hwang and S. Das Sarma, "Linear-in-T resistivity in dilute metals: A Fermi liquid perspective," Phys. Rev. B **99**, 085105 (2019).
